# Supplementary material for: Semi-Supervised Surface Anomaly Detection of Composite Wind Turbine Blades From Drone Imagery
Source: arXiv:2112.00556 source file (2021-12-01)
Supplement: Supplementary file 1 [file 10_appendix.tex]

\section*{\uppercase{Appendix}}

If any, the appendix should appear directly after the
references without numbering, and not on a new page. To do so please use the following command:
\textit{$\backslash$section*\{APPENDIX\}}
